# Supplementary material for: The Q-AMOEBA (CF) Polarizable Potential
Source: arXiv:2502.12708 ancillary file (2025-05-11)
Supplement: Supplementary file 1 [file QAMOEBA-CF-SupInfo.pdf]

# Supplementary Information: The Q-AMOEBA (CF) Polarizable Potential

Nastasia Mauger,<sup>1,2</sup> Thomas Plé,<sup>1</sup> Louis Lagardère,<sup>1</sup> Simon Huppert,<sup>3</sup> and Jean-Philip Piquemal<sup>1</sup>

<sup>1</sup>*Sorbonne Université, Laboratoire de Chimie Théorique, UMR 7616 CNRS, 75005, Paris, France*

<sup>2</sup>*Department of Chemistry, University of Pittsburgh, Pittsburgh, Pennsylvania 15260, United States*

<sup>3</sup>*Sorbonne Université, Institut des NanoSciences de Paris, UMR 7588 CNRS, 75005, Paris, France*

## CONTENTS

|                                                                                     |    |
|-------------------------------------------------------------------------------------|----|
| I. Simulation parameters for liquid water                                           | 2  |
| II. Initial and Optimized Parameters of the Q-AMOEBA water models                   | 2  |
| A. Average O-H bond and H-O-H in gas and liquid phase                               | 3  |
| B. Q-AMOEBA (2024) Force Field Parameters                                           | 4  |
| 1. adQTB method                                                                     | 4  |
| 2. PIMD method                                                                      | 7  |
| C. Q-AMOEBA (CF) Force Field Parameters                                             | 10 |
| 1. adQTB method                                                                     | 10 |
| 2. PIMD method                                                                      | 13 |
| III. Binding Energies of Water Clusters                                             | 16 |
| A. Binding Energies of the 10 Smith Dimers                                          | 16 |
| B. Binding Energies of trimer to 20-mers                                            | 17 |
| IV. Structural Properties of Liquid Water                                           | 18 |
| A. Radial Distribution Function                                                     | 18 |
| B. Average Energy Contributions                                                     | 19 |
| C. IR Absorption Spectra                                                            | 19 |
| V. Thermodynamic Properties                                                         | 21 |
| A. Liquid Properties                                                                | 21 |
| B. Molecular Dipole Moments                                                         | 22 |
| C. Heavy Water                                                                      | 22 |
| D. Ice I <sub>c</sub>                                                               | 22 |
| VI. Hydration Free Energies                                                         | 24 |
| A. Simulation parameters                                                            | 24 |
| B. Window parameters                                                                | 24 |
| C. Water and ions results                                                           | 24 |
| D. Small organic molecules results                                                  | 25 |
| VII. The Alanine Dipeptide                                                          | 27 |
| A. Simulation Parameters                                                            | 27 |
| B. Colvar Input File                                                                | 27 |
| C. adQTB and PIMD 2D Potential of Mean Force                                        | 28 |
| D. PMF difference between adQTB and PIMD parameters                                 | 28 |
| E. PMF difference between H <sub>2</sub> O and D <sub>2</sub> O solvents with adQTB | 29 |
| F. $\lambda$ -ABF Curves of the different components in the Solvation Free Energy   | 29 |
| G. Solvation Free Energy Decomposition                                              | 30 |
| H. Solvation Free Energy                                                            | 30 |
| References                                                                          | 31 |

## I. SIMULATION PARAMETERS FOR LIQUID WATER

The simulations were done at 1 atm in a cubic box with a size of 49.323 Å, containing 4000 molecules under periodic boundary conditions. The van der Waals (vdW) cutoff was set to 12 Å, and electrostatic interactions were calculated using the Smooth Particle Mesh Ewald (SPME) method [1] with a real-space cutoff of 7 Å and a  $60 \times 60 \times 60$  grid. A BAOAB-RESPA integrator was used, employing time steps of 0.2 fs for bonded interactions and 2 fs for nonbonded interactions. For PIMD simulations, 32 beads were used with the TRPMD method, utilizing a mild Langevin thermostat on the centroid with a friction coefficient of  $\gamma = 1 \text{ ps}^{-1}$ . In contrast, the adQTB method used a higher friction coefficient of  $20 \text{ ps}^{-1}$ . All thermodynamic properties presented in Section V were computed from 50 ns simulations to ensure convergence. Results in Section IV were done from 5 ns simulations.

## II. INITIAL AND OPTIMIZED PARAMETERS OF THE Q-AMOEBA WATER MODELS

In table I, we provide the set of parameters for the optimized Q-AMOEBA force fields, compared to the original AMOEBA-03 [2] values. Only the parameters that have been modified with respect to the original model are reported. The table provides values for 2 different models: Q-AMOEBA (CF) includes a charge flux term and is the model discussed in the main text, but we also provide refined parameter values in the case where CF is not included. This improved Q-AMOEBA force field (without CF) is referred to as Q-AMOEBA (2024) in the following, to distinguish it from our previous Q-AMOEBA model [3]. In addition, different approaches for the treatment of NQE lead to slightly different values for the liquid water density. Therefore two distinct Van der Waals parameter sets were developed: one to be used with the adQTB method, and another for the PIMD (indicated in parenthesis in table I). The core of the article focuses on the Q-AMOEBA (CF) results obtained with adQTB (with the appropriate set of parameters), while here, we provide all the results for the other parameters and for both adQTB and PIMD simulations.

| term   | parameter           | unit                                    | AMOEBA-03 | Q-AMOEBA (2024)     | Q-AMOEBA (CF)       |
|--------|---------------------|-----------------------------------------|-----------|---------------------|---------------------|
| vdW    | O vdW diameter      | Å                                       | 3.4050    | 3.409598 (3.412598) | 3.408598 (3.404698) |
|        | O vdW epsilon       | kcal.mol <sup>-1</sup>                  | 0.1100    | 0.113990 (0.124696) | 0.113890 (0.113890) |
|        | H vdW diameter      | Å                                       | 2.6550    | 2.645689 (2.603687) | 2.612686 (2.620387) |
|        | H vdW epsilon       | kcal.mol <sup>-1</sup>                  | 0.0135    | 0.010014 (0.010109) | 0.010065 (0.010625) |
|        | H vdW reduction     | none                                    | 0.910     | 0.937508 (0.940408) | 0.942308 (0.94911)  |
| bonded | O-H bond length     | Å                                       | 0.9572    | 0.9472 (0.9572)     | 0.9572 (0.9572)     |
|        | H-O-H angle         | Å                                       | 108.50    | 106.50 (107.50)     | 104.50 (104.50)     |
|        | bond force constant | kcal.mol <sup>-1</sup> .Å <sup>-2</sup> | 556.85    | 526.85 (526.85)     | 526.85 (526.85)     |

TABLE I: Value of the initial/AMOEBA-03 [2] water parameters compared to the new ones. The values in parenthesis are the one optimized for the PIMD method

### A. Average O-H bond and H-O-H in gas and liquid phase

|                 | Gas Phase     |                      | Liquid Phase  |                      |
|-----------------|---------------|----------------------|---------------|----------------------|
|                 | $r_{OH}$ (Å)  | $\theta_{HOH}$ (deg) | $r_{OH}$ (Å)  | $\theta_{HOH}$ (deg) |
| Q-AMOEBA (2024) | 0.947 (0.957) | 106.50 (107.50)      | 0.976 (0.986) | 105.30 (106.43)      |
| Q-AMOEBA (CF)   | 0.957         | 104.50               | 0.983         | 105.15 (105.13)      |
| AMOEBA-03       | 0.957         | 108.50               | 0.968         | 106.10               |
| Exp.            | 0.957         | 104.52               | 0.97          | 105.1                |

TABLE II: Average O-H bond length and H-O-H angle obtained in molecular dynamics simulations using Q-AMOEBA (2024) and Q-AMOEBA (CF) compared to original AMOEBA-03 model and experimental results [4, 5]. The main values correspond to adQTB simulations (or to classical MD simulations for the AMOEBA-03 model), and the values in parenthesis are obtained with the parameters set optimized for the PIMD method. If no value are given in parenthesis it indicates that adQTB and PIMD yield identical results. Note in particular that this is the case for the Q-AMOEBA (CF) model.

## B. Q-AMOEBA (2024) Force Field Parameters

### 1. *adQTB* method

```
forcefield      AMOEBA-WATER

bond-cubic      -2.55
bond-quartic     3.793125
angle-cubic      -0.014
angle-quartic    0.000056
angle-pentic     -0.0000007
angle-sextic     0.000000022
vdwtype         BUFFERED-14-7
radiusrule      CUBIC-MEAN
radiustype      R-MIN
radiussize      DIAMETER
epsilon         HHG
dielectric       1.0
polarization    MUTUAL
```

```
#####
##                               ##
## Literature References  ##
##                               ##
#####
```

P. Ren and J. W. Ponder, "A Polarizable Atomic Multipole Water Model for Molecular Mechanics Simulation", J. Phys. Chem. B, 107, 5933-5947 (2003)

Y. Kong, "Multipole Electrostatic Methods for Protein Modeling with Reaction Field Treatment", Ph.D. thesis, DBBS Program in Molecular Biophysics, Washington University, St. Louis, August, 1997 [available online from <http://dasher.wustl.edu/ponder/>]

alternative valence parameters to match symmetric and antisymmetric bond stretches by David Semrouni, Ecole Polytechnique, Paris

```
#####
##                               ##
## Atom Type Definitions  ##
##                               ##
#####
```

|      |   |   |   |                  |   |        |   |
|------|---|---|---|------------------|---|--------|---|
| atom | 1 | 1 | O | "AMOEBA Water O" | 8 | 15.995 | 2 |
| atom | 2 | 2 | H | "AMOEBA Water H" | 1 | 1.008  | 1 |

```
#####
##                               ##
## Van der Waals Parameters  ##
##                               ##
#####
```

|     |   |                    |                    |
|-----|---|--------------------|--------------------|
| vdw | 1 | 3.409598077410e+00 | 1.139901058311e-01 |
|-----|---|--------------------|--------------------|

|     |   |                    |                    |                    |
|-----|---|--------------------|--------------------|--------------------|
| vdw | 2 | 2.645686815889e+00 | 1.001445491727e-02 | 9.375081382906e-01 |
|-----|---|--------------------|--------------------|--------------------|

```
#####
##                               ##
## Bond Stretching Parameters  ##
##                               ##
#####
```

|      |   |   |        |        |
|------|---|---|--------|--------|
| bond | 1 | 2 | 526.85 | 0.9472 |
|------|---|---|--------|--------|

```
#####
##                               ##
## Angle Bending Parameters    ##
##                               ##
#####
```

|       |   |   |   |       |        |
|-------|---|---|---|-------|--------|
| angle | 2 | 1 | 2 | 48.70 | 106.50 |
|-------|---|---|---|-------|--------|

```
#####
##                               ##
## Urey-Bradley Parameters     ##
##                               ##
#####
```

|          |   |   |   |       |        |
|----------|---|---|---|-------|--------|
| ureybrad | 2 | 1 | 2 | -7.60 | 1.5337 |
|----------|---|---|---|-------|--------|

```
#####
##                               ##
## Atomic Multipole Parameters ##
##                               ##
#####
```

|           |   |    |    |          |          |         |
|-----------|---|----|----|----------|----------|---------|
| multipole | 1 | -2 | -2 | -0.51966 |          |         |
|           |   |    |    | 0.00000  | 0.00000  | 0.14279 |
|           |   |    |    | 0.37928  |          |         |
|           |   |    |    | 0.00000  | -0.41809 |         |
|           |   |    |    | 0.00000  | 0.00000  | 0.03881 |

|           |   |   |   |          |          |          |
|-----------|---|---|---|----------|----------|----------|
| multipole | 2 | 1 | 2 | 0.25983  |          |          |
|           |   |   |   | -0.03859 | 0.00000  | -0.05818 |
|           |   |   |   | -0.03673 |          |          |
|           |   |   |   | 0.00000  | -0.10739 |          |
|           |   |   |   | -0.00203 | 0.00000  | 0.14412  |

```
#####
##                               ##
## Dipole Polarizability Parameters ##
##                               ##
#####
```

|          |   |       |       |   |
|----------|---|-------|-------|---|
| polarize | 1 | 0.837 | 0.390 | 2 |
| polarize | 2 | 0.496 | 0.390 | 1 |

## 2. PIMD method

```

forcefield      AMOEBA-WATER

bond-cubic      -2.55
bond-quartic    3.793125
angle-cubic     -0.014
angle-quartic   0.000056
angle-pentic    -0.0000007
angle-sextic    0.000000022
vdwtype         BUFFERED-14-7
radiusrule      CUBIC-MEAN
radiustype      R-MIN
radiussize      DIAMETER
epsilonrule     HHG
dielectric      1.0
polarization    MUTUAL

```

```

#####
##                               ##
## Literature References         ##
##                               ##
#####

```

P. Ren and J. W. Ponder, "A Polarizable Atomic Multipole Water Model for Molecular Mechanics Simulation", J. Phys. Chem. B, 107, 5933-5947 (2003)

Y. Kong, "Multipole Electrostatic Methods for Protein Modeling with Reaction Field Treatment", Ph.D. thesis, DBBS Program in Molecular Biophysics, Washington University, St. Louis, August, 1997 [available online from <http://dasher.wustl.edu/ponder/>]

alternative valence parameters to match symmetric and antisymmetric bond stretches by David Semrouni, Ecole Polytechnique, Paris

```

#####
##                               ##
## Atom Type Definitions         ##
##                               ##
#####

```

|      |   |   |   |                  |   |        |   |
|------|---|---|---|------------------|---|--------|---|
| atom | 1 | 1 | O | "AMOEBA Water O" | 8 | 15.995 | 2 |
| atom | 2 | 2 | H | "AMOEBA Water H" | 1 | 1.008  | 1 |

```

#####
##                               ##
## Van der Waals Parameters     ##
##                               ##
#####

```

|     |   |                    |                    |                    |
|-----|---|--------------------|--------------------|--------------------|
| vdw | 1 | 3.412598077410e+00 | 1.246961058311e-01 |                    |
| vdw | 2 | 2.603686815889e+00 | 1.010945491727e-02 | 9.404081382906e-01 |

```
#####
##                               ##
## Bond Stretching Parameters ##
##                               ##
#####
```

```
bond      1      2      526.85      0.9572
```

```
#####
##                               ##
## Angle Bending Parameters  ##
##                               ##
#####
```

```
angle      2      1      2      48.70      107.50
```

```
#####
##                               ##
## Urey-Bradley Parameters  ##
##                               ##
#####
```

```
ureybrad    2      1      2      -7.60      1.5337
```

```
#####
##                               ##
## Atomic Multipole Parameters ##
##                               ##
#####
```

```
multipole    1    -2    -2
              -0.51966
              0.00000      0.00000      0.14279
              0.37928
              0.00000     -0.41809
              0.00000      0.00000      0.03881
```

```
multipole    2      1      2
              0.25983
             -0.03859      0.00000     -0.05818
             -0.03673
              0.00000     -0.10739
             -0.00203      0.00000      0.14412
```

```
#####
##                               ##
## Dipole Polarizability Parameters ##
##                               ##
#####
```



|          |   |       |       |   |
|----------|---|-------|-------|---|
| polarize | 1 | 0.837 | 0.390 | 2 |
| polarize | 2 | 0.496 | 0.390 | 1 |

## C. Q-AMOEBA (CF) Force Field Parameters

### 1. *adQTB method*

```
forcefield      AMOEBA-WATER

bond-cubic      -2.55
bond-quartic    3.793125
angle-cubic     -0.014
angle-quartic   0.000056
angle-pentic    -0.0000007
angle-sextic    0.000000022
vdwtype        BUFFERED-14-7
radiusrule     CUBIC-MEAN
radiustype     R-MIN
radiussize     DIAMETER
epsilon rule    HHG
dielectric      1.0
polarization    MUTUAL
```

```
#####
##                               ##
## Literature References        ##
##                               ##
#####
```

P. Ren and J. W. Ponder, "A Polarizable Atomic Multipole Water Model for Molecular Mechanics Simulation", J. Phys. Chem. B, 107, 5933-5947 (2003)

Y. Kong, "Multipole Electrostatic Methods for Protein Modeling with Reaction Field Treatment", Ph.D. thesis, DBBS Program in Molecular Biophysics, Washington University, St. Louis, August, 1997 [available online from <http://dasher.wustl.edu/ponder/>]

alternative valence parameters to match symmetric and antisymmetric bond stretches by David Semrouni, Ecole Polytechnique, Paris

```
#####
##                               ##
## Atom Type Definitions      ##
##                               ##
#####
```

|      |   |   |   |                  |   |        |   |
|------|---|---|---|------------------|---|--------|---|
| atom | 1 | 1 | O | "AMOEBA Water O" | 8 | 15.995 | 2 |
| atom | 2 | 2 | H | "AMOEBA Water H" | 1 | 1.008  | 1 |

```
#####
##                               ##
## Van der Waals Parameters  ##
##                               ##
#####
```

|     |   |                    |                    |
|-----|---|--------------------|--------------------|
| vdw | 1 | 3.408598077410e+00 | 1.138901058311e-01 |
|-----|---|--------------------|--------------------|

|     |   |                    |                    |                    |
|-----|---|--------------------|--------------------|--------------------|
| vdw | 2 | 2.612686815889e+00 | 1.006645491727e-02 | 9.423081382906e-01 |
|-----|---|--------------------|--------------------|--------------------|

```
#####
##                               ##
## Bond Stretching Parameters  ##
##                               ##
#####
```

|      |   |   |        |        |
|------|---|---|--------|--------|
| bond | 1 | 2 | 526.85 | 0.9572 |
|------|---|---|--------|--------|

```
#####
##                               ##
## Angle Bending Parameters    ##
##                               ##
#####
```

|       |   |   |   |       |        |
|-------|---|---|---|-------|--------|
| angle | 2 | 1 | 2 | 48.70 | 104.50 |
|-------|---|---|---|-------|--------|

```
#####
##                               ##
## Urey-Bradley Parameters     ##
##                               ##
#####
```

|          |   |   |   |       |        |
|----------|---|---|---|-------|--------|
| ureybrad | 2 | 1 | 2 | -7.60 | 1.5337 |
|----------|---|---|---|-------|--------|

```
#####
##                               ##
## Atomic Multipole Parameters ##
##                               ##
#####
```

|           |   |    |    |          |          |         |
|-----------|---|----|----|----------|----------|---------|
| multipole | 1 | -2 | -2 | -0.51966 |          |         |
|           |   |    |    | 0.00000  | 0.00000  | 0.14279 |
|           |   |    |    | 0.37928  |          |         |
|           |   |    |    | 0.00000  | -0.41809 |         |
|           |   |    |    | 0.00000  | 0.00000  | 0.03881 |

|           |   |   |   |          |          |          |
|-----------|---|---|---|----------|----------|----------|
| multipole | 2 | 1 | 2 | 0.25983  |          |          |
|           |   |   |   | -0.03859 | 0.00000  | -0.05818 |
|           |   |   |   | -0.03673 |          |          |
|           |   |   |   | 0.00000  | -0.10739 |          |
|           |   |   |   | -0.00203 | 0.00000  | 0.14412  |

```
#####
##                               ##
## Dipole Polarizability Parameters ##
##                               ##
#####
```

|          |   |       |       |   |
|----------|---|-------|-------|---|
| polarize | 1 | 0.837 | 0.390 | 2 |
| polarize | 2 | 0.496 | 0.390 | 1 |

```
#####
##                               ##
## Charge Flux Parameters      ##
##                               ##
#####
```

```
#####
##                               ##
## angle charge flux parameters multiplied by radian to ##
## change e-/deg used by Pengyu Ren group to e-/radian ##
##                               ##
#####
```

|          |   |   |   |         |        |         |         |
|----------|---|---|---|---------|--------|---------|---------|
| bndcflux | 1 | 2 |   | -0.0303 |        |         |         |
| angcflux | 2 | 1 | 2 | 0.0433  | 0.0433 | -0.0453 | -0.0453 |

## 2. PIMD method

```
forcefield      AMOEBA-WATER

bond-cubic      -2.55
bond-quartic    3.793125
angle-cubic     -0.014
angle-quartic   0.000056
angle-pentic    -0.0000007
angle-sextic    0.000000022
vdwtype         BUFFERED-14-7
radiusrule      CUBIC-MEAN
radiustype      R-MIN
radiussize      DIAMETER
epsilonrule     HHG
dielectric      1.0
polarization    MUTUAL
```

```
#####
##                               ##
## Literature References        ##
##                               ##
#####
```

P. Ren and J. W. Ponder, "A Polarizable Atomic Multipole Water Model for Molecular Mechanics Simulation", J. Phys. Chem. B, 107, 5933-5947 (2003)

Y. Kong, "Multipole Electrostatic Methods for Protein Modeling with Reaction Field Treatment", Ph.D. thesis, DBBS Program in Molecular Biophysics, Washington University, St. Louis, August, 1997 [available online from <http://dasher.wustl.edu/ponder/>]

alternative valence parameters to match symmetric and antisymmetric bond stretches by David Semrouni, Ecole Polytechnique, Paris

```
#####
##                               ##
## Atom Type Definitions        ##
##                               ##
#####
```

|      |   |   |   |                  |   |        |   |
|------|---|---|---|------------------|---|--------|---|
| atom | 1 | 1 | O | "AMOEBA Water O" | 8 | 15.995 | 2 |
| atom | 2 | 2 | H | "AMOEBA Water H" | 1 | 1.008  | 1 |

```
#####
##                               ##
## Van der Waals Parameters      ##
##                               ##
#####
```

|     |   |                    |                    |                    |
|-----|---|--------------------|--------------------|--------------------|
| vdw | 1 | 3.404698077410e+00 | 1.138901058311e-01 |                    |
| vdw | 2 | 2.620386815889e+00 | 1.016245591727e-02 | 9.491101382906e-01 |

```
#####
##                               ##
## Bond Stretching Parameters  ##
##                               ##
#####
```

```
bond      1      2      526.85      0.9572
```

```
#####
##                               ##
## Angle Bending Parameters  ##
##                               ##
#####
```

```
angle     2      1      2      48.70      104.50
```

```
#####
##                               ##
## Urey-Bradley Parameters  ##
##                               ##
#####
```

```
ureybrad  2      1      2      -7.60      1.5337
```

```
#####
##                               ##
## Atomic Multipole Parameters  ##
##                               ##
#####
```

```
multipole  1     -2     -2      -0.51966
              0.00000      0.00000      0.14279
              0.37928
              0.00000     -0.41809
              0.00000      0.00000      0.03881
```

```
multipole  2      1      2      0.25983
              -0.03859      0.00000     -0.05818
              -0.03673
              0.00000     -0.10739
              -0.00203      0.00000      0.14412
```

```
#####
##                               ##
## Dipole Polarizability Parameters  ##
##                               ##
#####
```

|          |   |       |       |   |
|----------|---|-------|-------|---|
| polarize | 1 | 0.837 | 0.390 | 2 |
| polarize | 2 | 0.496 | 0.390 | 1 |

```
#####
##                               ##
## Charge Flux Parameters      ##
##                               ##
#####
```

```
#####
##                               ##
## angle charge flux parameters multiplied by radian to ##
## change e-/deg used by Pengyu Ren group to e-/radian ##
##                               ##
#####
```

|          |   |   |   |         |        |         |         |
|----------|---|---|---|---------|--------|---------|---------|
| bndcflux | 1 | 2 |   | -0.0303 |        |         |         |
| angcflux | 2 | 1 | 2 | 0.0433  | 0.0433 | -0.0453 | -0.0453 |

### III. BINDING ENERGIES OF WATER CLUSTERS

#### A. Binding Energies of the 10 Smith Dimers

| (H <sub>2</sub> O) <sub>2</sub> | CCSD(T) | AMOEBA-03 | Q-AMOEBA (2024) | Q-AMOEBA (CF) |
|---------------------------------|---------|-----------|-----------------|---------------|
| Smith01                         | -4.97   | -4.58     | -4.87           | -5.22         |
| Smith02                         | -4.45   | -3.98     | -4.29           | -4.62         |
| Smith03                         | -4.42   | -3.94     | -4.25           | -4.57         |
| Smith04                         | -4.25   | -3.54     | -3.41           | -3.77         |
| Smith05                         | -4.00   | -2.69     | -2.98           | -3.35         |
| Smith06                         | -3.96   | -2.59     | -2.88           | -3.25         |
| Smith07                         | -3.26   | -2.55     | -2.71           | -3.05         |
| Smith08                         | -1.30   | -0.8      | -0.93           | -1.26         |
| Smith09                         | -3.05   | -2.69     | -2.87           | -3.21         |
| Smith10                         | -2.18   | -1.89     | -2.04           | -2.36         |
| RMSE                            |         | 0.81      | 0.59 (0.58)     | 0.37 (0.37)   |

TABLE III: Binding Energies of the 10 Smith dimers using Q-AMOEBA (2024) and Q-AMOEBA (CF) compared to the AMOEBA-03 model and *ab initio* references. The values in parenthesis are the RMSE obtained with the parameter set optimized for the PIMD method. CCSD(T)/CBS results come from reference [6].



## B. Binding Energies of trimer to 20-mers

| $(\text{H}_2\text{O})_n$ | geometry            | QM      | AMOEBA-03 | Q-AMOEBA (2024) | Q-AMOEBA (CF) |
|--------------------------|---------------------|---------|-----------|-----------------|---------------|
| n=3                      | cyclic              | -15.74  | -15.03    | -16.01          | -16.17        |
| n=4                      | cyclic              | -27.40  | -27.63    | -29.06          | -29.37        |
| n=5                      | cyclic              | -35.93  | -36.38    | -38.36          | -38.65        |
| n=6                      | prism               | -45.92  | -45.71    | -47.93          | -47.09        |
|                          | cage                | -45.67  | -45.82    | -47.97          | -48.13        |
|                          | bag                 | -44.30  | -44.79    | -47.10          | -46.98        |
|                          | cyclic chair        | -44.12  | -44.62    | -47.13          | -47.46        |
|                          | book1               | -45.20  | -45.6     | -47.93          | -48.22        |
|                          | book2               | -44.90  | -45.37    | -47.67          | -47.88        |
|                          | cyclic boat1        | -43.13  | -43.78    | -46.20          | -46.44        |
|                          | cyclic boat2        | -43.07  | -43.84    | -46.27          | -46.57        |
| n=8                      | S4                  | -72.70  | -72.34    | -75.76          | -76.00        |
|                          | D2d                 | -72.70  | -72.39    | -75.80          | -76.04        |
| n=11                     | 434                 | -105.72 | -101.74   | -106.55         | -106.29       |
|                          | 515                 | -105.18 | -102.08   | -107.07         | -106.45       |
|                          | 551                 | -104.92 | -101.85   | -106.84         | -106.58       |
|                          | 443                 | -104.76 | -101.86   | -106.75         | -106.95       |
|                          | 4412                | -103.97 | -101.41   | -106.49         | -106.67       |
| n=16                     | boat-a              | -170.80 | -161.21   | -168.99         | -169.17       |
|                          | boat-b              | -170.63 | -161.54   | -169.32         | -169.41       |
|                          | antiboat            | -170.54 | -162.26   | -170.30         | -171.05       |
|                          | ABAB                | -171.05 | -161.18   | -168.72         | -170.26       |
|                          | AABB                | -170.51 | -160.98   | -168.55         | -170.12       |
| n=17                     | sphere              | -182.54 | -173.02   | -181.51         | -181.99       |
|                          | 5525                | -181.83 | -172.32   | -180.76         | -181.01       |
| n=20                     | dodecahedron        | -200.10 | -197.03   | -206.56         | -203.67       |
|                          | fused cubes         | -212.10 | -205.76   | -215.38         | -217.52       |
|                          | face sharing prisms | -215.20 | -206.13   | -215.96         | -217.60       |
|                          | edge sharing prisms | -218.10 | -208.46   | -218.72         | -219.62       |
| RMSE                     |                     |         | 3.33      | 2.47 (2.20)     | 2.45 (2.35)   |

TABLE IV: Binding Energies of trimer to 20-mer of water clusters computed using Q-AMOEBA (2024) and Q-AMOEBA (CF) models compared to AMOEBA-03 and *ab initio* data. The values in parenthesis are the RMSE obtained with the parameter set optimized for the PIMD method. QM reference correspond to CCSD(T)/CBS for  $n \leq 6$  [7, 8] and to MP2/CBS for  $n \geq 8$  [9–11].

## IV. STRUCTURAL PROPERTIES OF LIQUID WATER

### A. Radial Distribution Function

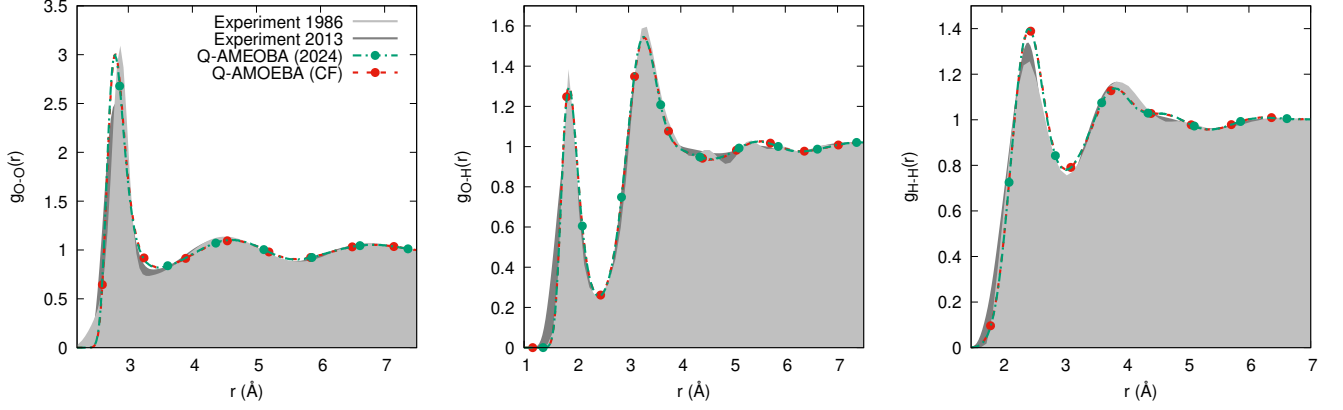

FIG. 1: RDFs computed at 298.15K with Q-AMOEBA (2024) and Q-AMOEBA (CF) compared to the X-ray (2013) using adQTB set of parameters [12] and neutron (1986) [4] diffraction experiments.

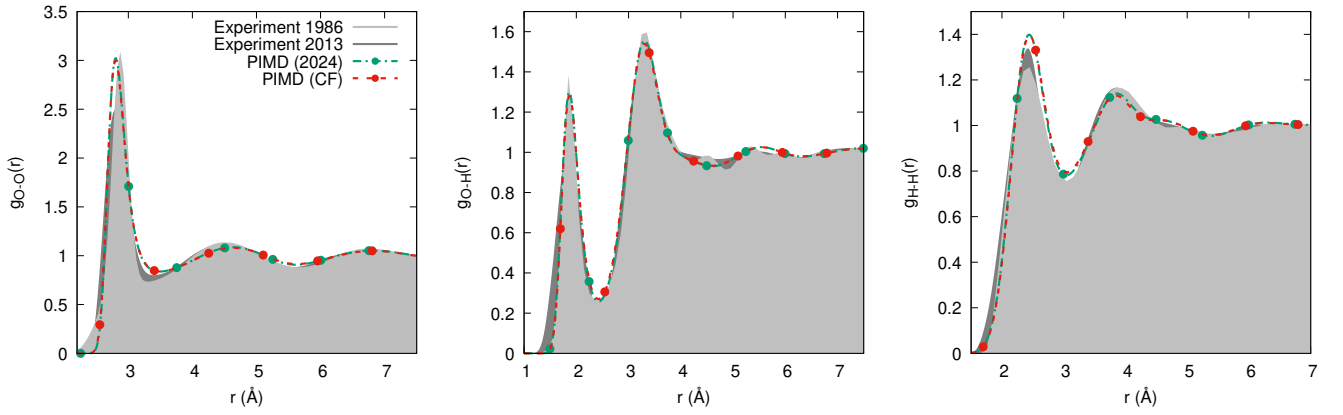

FIG. 2: RDFs computed at 298.15K with Q-AMOEBA (2024) and Q-AMOEBA (CF) compared to the X-ray (2013) using PIMD set of parameters [12] and neutron (1986) [4] diffraction experiments.

## B. Average Energy Contributions

|                 | Bond stretching | Angle bending | Urey-Bradley | Van der Waals | Atomic Multipoles | Polarization | Non-Bonded |
|-----------------|-----------------|---------------|--------------|---------------|-------------------|--------------|------------|
| Q-AMOEBA (2024) | 5.40            | 1.23          | -0.11        | 4.38          | -9.85             | -4.36        | -9.83      |
| Q-AMOEBA (CF)   | 5.31            | 1.14          | -0.12        | 4.36          | -9.94             | -4.41        | -9.99      |
| PIMD (2024)     | 5.31            | 1.19          | -0.12        | 4.24          | -9.80             | -4.30        | -9.86      |
| PIMD (CF)       | 5.18            | 1.13          | -0.12        | 4.20          | -9.73             | -4.26        | -9.79      |
| AMOEBA-03       | 0.73            | 0.40          | -0.02        | 4.41          | -10.17            | -4.34        | -10.1      |

TABLE V: Average energy contributions of Q-AMOEBA (2024) and Q-AMOEBA (CF) obtained with the adQTB and the PIMD methods (using their specific set of parameters in each case), at a temperature of 298.15K. All energies are given in kcal.mol<sup>-1</sup> per water molecule and obtained from 5 ns simulations at constant volume corresponding to the density  $\rho = 0.997$  g.cm<sup>-3</sup>.

## C. IR Absorption Spectra

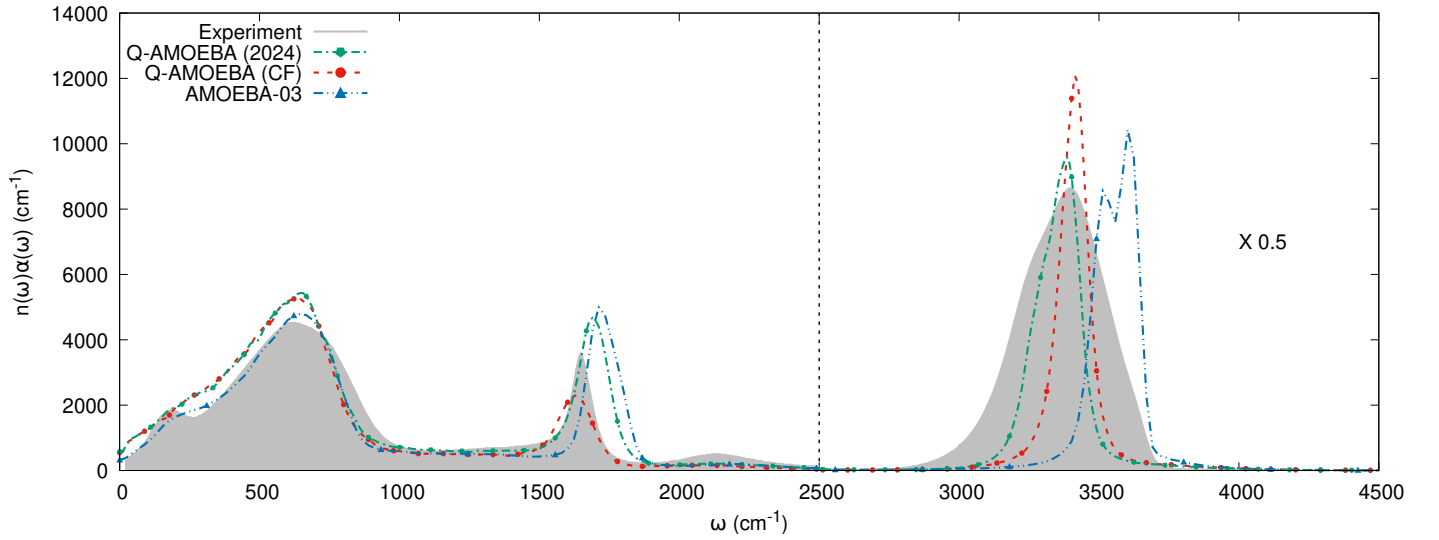

FIG. 3: IR absorption spectra computed at 300 K and  $\rho = 0.997$  g.cm<sup>-3</sup> with the Q-AMOEBA (2024) and Q-AMOEBA (CF) using the adQTB method and the corresponding set of parameters. They are compared with AMOEBA-03 (classical MD) and experimental data [13]. The right part of the plot, corresponding to the stretching mode multiplied by 0.5.

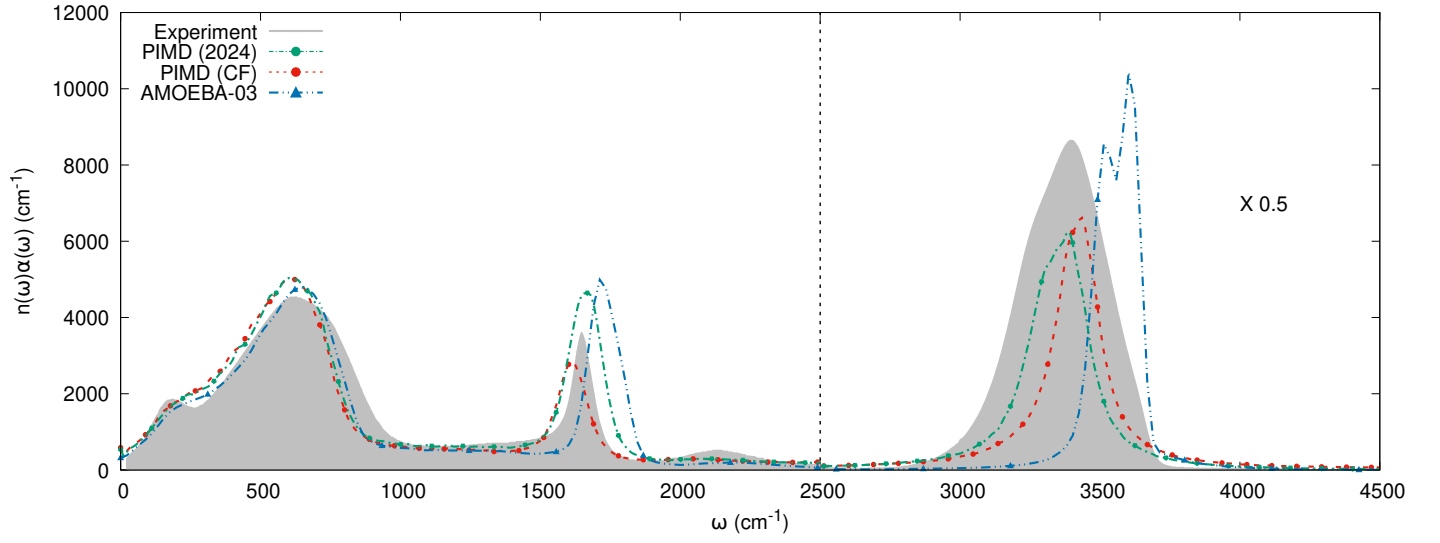

FIG. 4: IR absorption spectra computed at 300 K and  $\rho = 0.997 \text{ g.cm}^{-3}$  with the Q-AMOEBA (2024) and Q-AMOEBA (CF) using the PIMD method and the corresponding set of parameters. They are compared with AMOEBA-03 (classical MD) and experimental data [13]. The right part of the plot, corresponding to the stretching mode multiplied by 0.5.

## V. THERMODYNAMIC PROPERTIES

### A. Liquid Properties

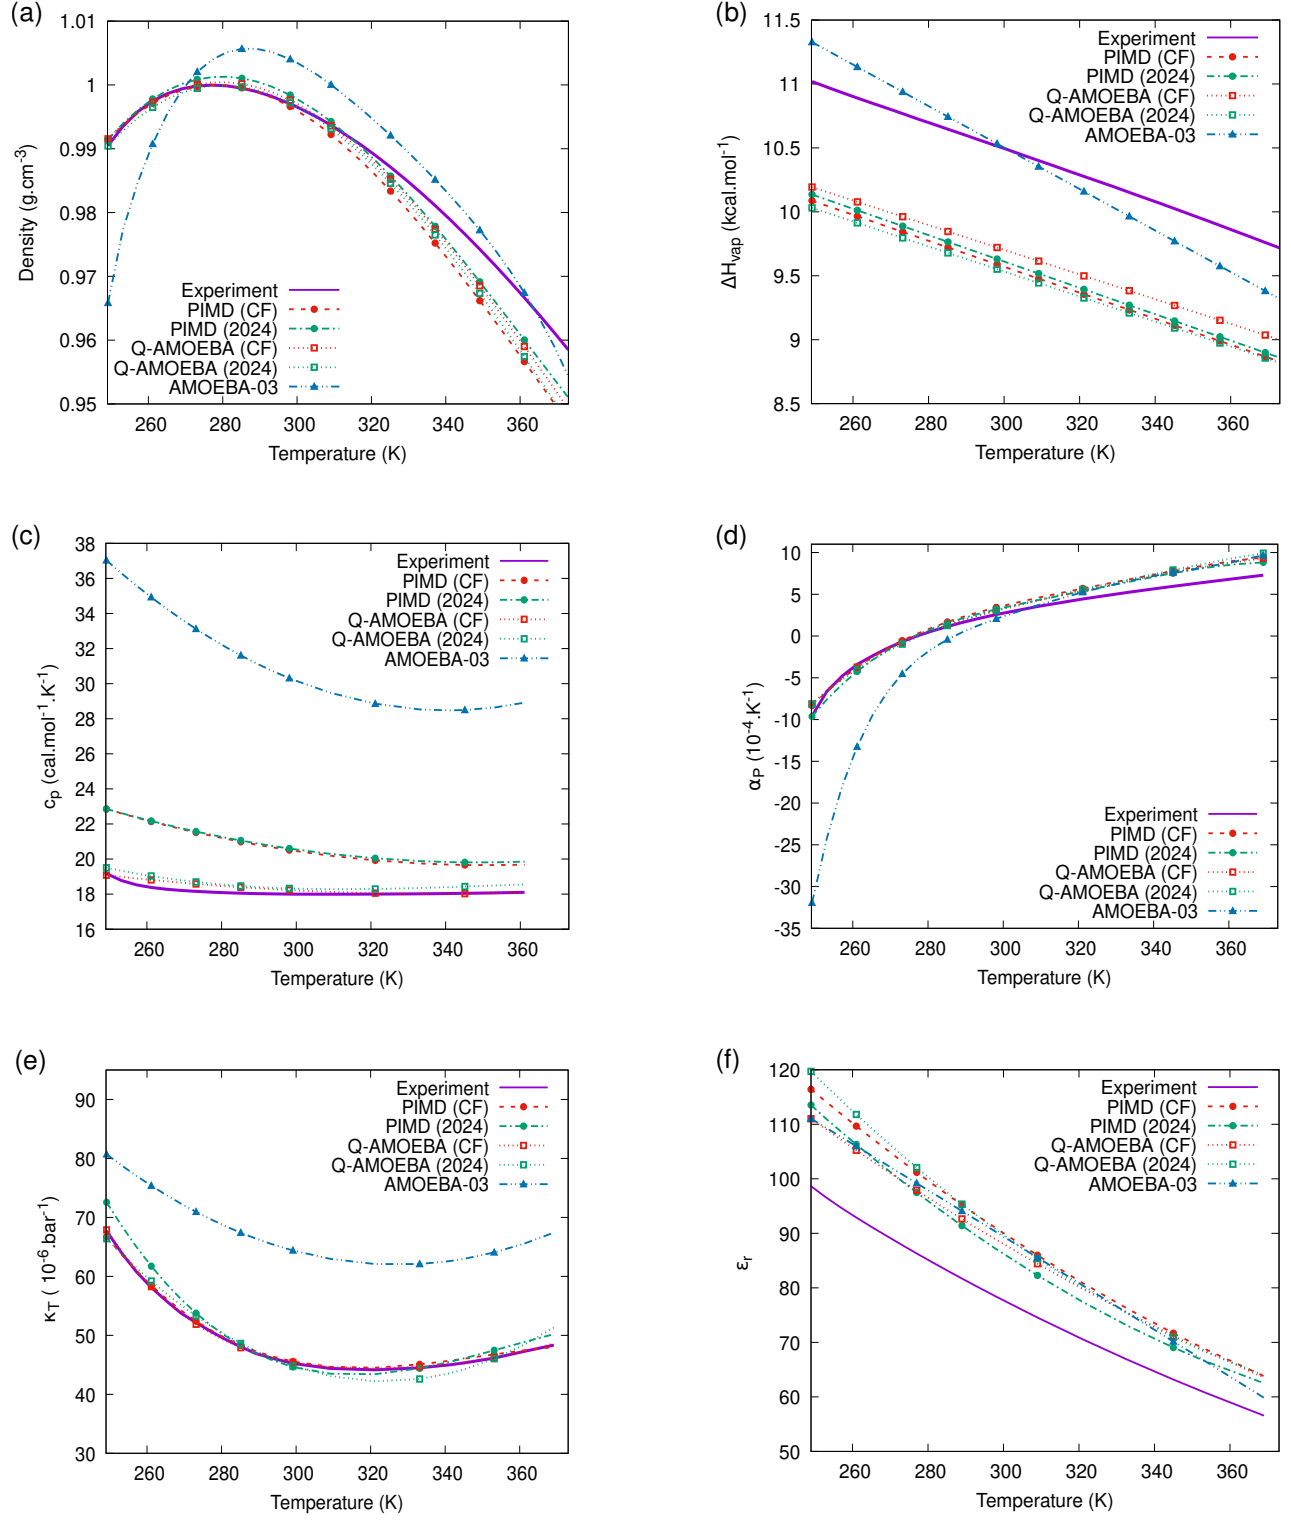

FIG. 5: Liquid properties of water at 1 atm pressure with Q-AMOEBA (2024) and Q-AMOEBA (CF) using adQTB and PIMD methods compared to AMOEBA-03 (classical MD) and experimental data [13–16].

## B. Molecular Dipole Moments

|                 | Gas Phase   | Liquid Phase                    |
|-----------------|-------------|---------------------------------|
| Q-AMOEBA (2024) | 1.79 (1.78) | 2.77 (2.75)                     |
| Q-AMOEBA (CF)   | 1.84 (1.84) | 2.77 (2.75)                     |
| AMOEBA-03       | 1.77        | 2.75                            |
| Experiments     | 1.85 [17]   | 2.9 $\pm$ 0.6 [18]<br>2.95 [19] |

TABLE VI: Molecular dipole moments at 298.15 K in Debye with the different models using adQTB compared to experimental [17, 18] and *ab initio* MD [19] data. Values in parenthesis are the one obtained using the parameters sets optimized through PIMD method.

## C. Heavy Water

In the Born-Oppenheimer approximation, the PES is independent on the nuclei’s mass. Therefore in classical MD, equilibrium (time-independent) properties are completely independent on the isotopic species (hydrogen versus deuterium for instance), and isotope effects on dynamical (time-dependent) properties are generally limited. However, experiments show that isotope effects can have a notable impact a variety of properties such as reaction rates and equilibrium constants. For instance, D<sub>2</sub>O is toxic and can impact protein stability [20]. This cannot be captured by usual FF, which are fitted to implicitly compensate for errors due to the neglect of NQE in classical MD simulations, but only for the most common isotopic species (H<sub>2</sub>O in the case of water). This oversight can lead to significant inaccuracies in predicting the properties of water, and generally of systems where hydrogen bonds play a crucial role.

Table VII illustrates that quantum MD simulations (using adQTB or PIMD) with the Q-AMOEBA (CF) FF can qualitatively reflect the trends observed experimentally upon deuteration of water, unlike classical MD simulations with AMOEBA-03. In particular, Q-AMOEBA predicts a heat capacity  $c_p$  increase for deuterated water of approximately 3.4 kcal/mol compared to the experimental value of 2.2 kcal/mol. Our new models are also able to describe at least qualitatively the changes under deuteration for the enthalpy of vaporization  $\Delta H_{\text{vap}}$  with an increase of approximately 0.6 kcal.mol<sup>-1</sup>, to be compared to the experimental change of 0.3 kcal.mol<sup>-1</sup>.

|                 | H <sub>2</sub> O |            |        | D <sub>2</sub> O |            |        |
|-----------------|------------------|------------|--------|------------------|------------|--------|
|                 | $\rho$           | $\Delta H$ | $c_p$  | $\rho$           | $\Delta H$ | $c_p$  |
| Q-AMOEBA (2024) | 0.997            | 9.55       | 18.356 | 1.105            | 10.14      | 21.83  |
| Q-AMOEBA (CF)   | 0.998            | 9.72       | 18.229 | 1.105            | 10.30      | 21.544 |
| AMOEBA-03       | 1.0              | 10.5       | 33.9   | 1.1              | 10.4       | 30.5   |
| Exp.            | 0.997            | 10.52      | 18.002 | 1.104            | 10.85      | 20.148 |

TABLE VII: Thermodynamic properties computed at 298.15K under 1 atm pressure for adQTB simulations with the Q-AMOEBA (2024) and Q-AMOEBA (CF) models compared to classical MD simulations with AMOEBA-03 for H<sub>2</sub>O and D<sub>2</sub>O compared to experimental values [15, 21]. The density  $\rho$  is given in g.cm<sup>-3</sup>, the enthalpy of vaporization  $\Delta H_{\text{vap}}$  in kcal.mol<sup>-1</sup> and the isobaric heat capacity  $c_p$  in cal.mol<sup>-1</sup>.K<sup>-1</sup>.

## D. Ice I<sub>c</sub>

To further assess the transferability of Q-AMOEBA, we extended our study to investigate the density of ice phase I<sub>c</sub>. These simulations were conducted at 78 K under 0 atm pressure. The results showed that Q-AMOEBA (2024) and Q-AMOEBA (CF) produced densities of 0.904 g.cm<sup>-3</sup> and 0.901 g.cm<sup>-3</sup>, respectively. In comparison, the experimental value is 0.931 g.cm<sup>-3</sup>. However, running a PIMD simulation using AMOEBA-03 parameters with 128

beads underestimated the density by approximately 6.8%, highlighting the significant influence of atomic quantum delocalization effects on different water phases and the error compensations in the FF parameters. This implies that our Q-AMOEBA models demonstrate better agreement with experimental data for ice phase  $I_c$  density compared to the classical AMOEBA-03 model. Therefore, it might be valuable to include some ice phase properties in the fitting procedure to enhance the transferability of the model, a practice previously employed, for example, in the development of TIP4PQ/2005 [22].

## VI. HYDRATION FREE ENERGIES

### A. Simulation parameters

All hydration free energy calculations were performed using a free energy perturbation procedure based on multiple thermodynamic states within the  $NVT$  ensemble at 298.15 K. The detailed MD window parameters are provided in Tables VIII and IX. Each thermodynamic state was thermalized for 1.5 ns and simulated for 5 ns using a BAOAB-RESPA integrator with a bonded/nonbonded time-step split of 0.2 fs and 2 fs, respectively. The Bennett Acceptance Ratio (BAR) method [23] and the Path Integral BAR (PI-BAR) method for PIMD results [24] were then employed to estimate the free energy. The final free energy was obtained by summing the contributions from all windows, with an additional 1.9 kcal.mol<sup>-1</sup> added to each ion [25]. The solute parameters were the same as those used in [24], while the solvents were Q-AMOEBA (2024), Q-AMOEBA (CF), or AMOEBA-03. The box size, corresponding Ewald and vdW cutoffs, friction coefficients, and the number of beads used were consistent with those employed in the water calculations.

### B. Window parameters

| State no.               | 1   | 2   | 3   | 4   | 5   | 6   | 7   | 8   | 9   | 10  | 11  | 12  | 13  | 14  | 14-2 | 15  | 15-2 | 16  | 17  | 18  | 19  | 20  | 21  |
|-------------------------|-----|-----|-----|-----|-----|-----|-----|-----|-----|-----|-----|-----|-----|-----|------|-----|------|-----|-----|-----|-----|-----|-----|
| $\lambda_{\text{elec}}$ | 1.0 | 0.9 | 0.8 | 0.7 | 0.6 | 0.5 | 0.4 | 0.3 | 0.2 | 0.1 | 0.0 | 0.0 | 0.0 | 0.0 | 0.0  | 0.0 | 0.0  | 0.0 | 0.0 | 0.0 | 0.0 | 0.0 | 0.0 |
| $\lambda_{\text{vdW}}$  | 1.0 | 1.0 | 1.0 | 1.0 | 1.0 | 1.0 | 1.0 | 1.0 | 1.0 | 1.0 | 1.0 | 0.9 | 0.8 | 0.7 | 0.75 | 0.6 | 0.65 | 0.5 | 0.4 | 0.3 | 0.2 | 0.1 | 0.0 |

TABLE VIII: Decoupling window parameters used to compute the hydration free energies for water, ions, and small organic molecules. The 14-2 and 15-2 states correspond to the additional parameter windows used for calculating the hydration free energies of the small organic molecules.

| State no.               | 1   | 2   | 3   | 4   | 5   | 6   | 7   | 8   | 9   | 10  | 11  |
|-------------------------|-----|-----|-----|-----|-----|-----|-----|-----|-----|-----|-----|
| $\lambda_{\text{elec}}$ | 0.0 | 0.1 | 0.2 | 0.3 | 0.4 | 0.5 | 0.6 | 0.7 | 0.8 | 0.9 | 1.0 |

TABLE IX: Gas-phase recharge window parameters used to compute the hydration free energies for ions and small organic molecules.

### C. Water and ions results

|                 | H <sub>2</sub> O | F <sup>-</sup> | Na <sup>+</sup> | Mg <sup>2+</sup> | Cl <sup>-</sup> | K <sup>+</sup> | Ca <sup>2+</sup> | Br <sup>-</sup> | I <sup>-</sup> |
|-----------------|------------------|----------------|-----------------|------------------|-----------------|----------------|------------------|-----------------|----------------|
| Q-AMOEBA (2024) | -5.64 (-5.57)    | -116.1         | -88.4           | -427.8           | -86.1           | -71.3          | -351.3           | -79.8           | -71.1          |
| Q-AMOEBA CF     | -5.79 (-5.69)    | -116.1         | -88.5           | -427.7           | -85.7           | -71.4          | -351.2           | -79.6           | -70.8          |
| AMOEBA-03       | - 5.78           | -114.7         | -89.7           | -432.4           | -84.1           | -72.3          | -354.6           | -77.7           | -69.3          |
| Expt.           | -6.32            | -119.7         | -88.7           | -435             | -89.1           | -71.2          | -356.8           | -82.7           | -74.3          |

TABLE X: Hydration free energies of water and different ions given in kcal.mol<sup>-1</sup> obtained with Q-AMOEBA (2024) and Q-AMOEBA (CF) models compared to AMOEBA-03 and experiments [26]. The values in parenthesis are the values obtained with the parameters set optimized through the PIMD method. 1.9 kcal.mol<sup>-1</sup> was added to each of the simulated ion hydration solvation free energies [25]



#### D. Small organic molecules results

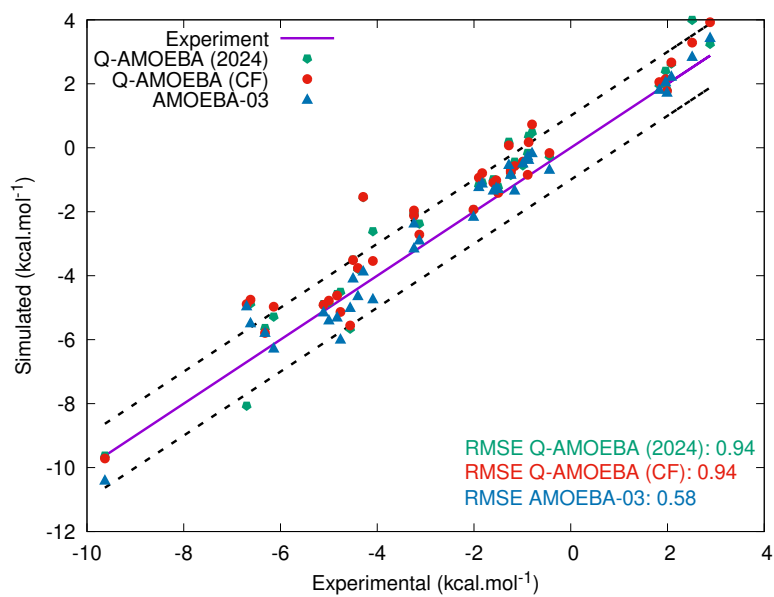

FIG. 6: Hydration free energies of small organic molecules using Q-AMOEBA (2024), Q-AMOEBA (CF) and AMOEBA-03 with their respective RMSE compared to experimental values. The dashed-lines represents the chemical accuracy.

|                      | Expt    | Q-AMOEBA (2024) | Q-AMOEBA (CF) | AMOEBA-03 |
|----------------------|---------|-----------------|---------------|-----------|
| imidazole            | -9.6300 | -9.6293         | -9.7145       | -10.4000  |
| aceticacid           | -6.700  | -8.0694         | -4.8873       | -4.9500   |
| phenol               | -6.6200 | -4.8747         | -4.7504       | -5.4800   |
| water                | -6.32   | -5.64           | -5.79         | -5.78     |
| p-cresol             | -6.1400 | -5.2841         | -4.9697       | -6.2700   |
| methanol             | -5.1100 | -4.8914         | -4.9128       | -5.1400   |
| ethanol              | -5.0000 | -4.8296         | -4.7805       | -5.3900   |
| propanol             | -4.8300 | -4.5777         | -4.6211       | -5.3000   |
| isopropanol          | -4.7600 | -4.5081         | -5.1337       | -5.9900   |
| methylamine          | -4.5600 | -5.6599         | -5.5568       | -5.000    |
| ethylamine           | -4.5000 | -3.5037         | -3.5109       | -4.0800   |
| propylamine          | -4.4000 | -3.7889         | -3.7588       | -4.6300   |
| dimethylamine        | -4.2900 | -1.5453         | -1.5365       | -3.8600   |
| Octan-1-ol           | -4.0900 | -2.6139         | -3.5399       | -4.7300   |
| trimethylamine       | -3.2400 | -2.0010         | -1.9615       | -2.3600   |
| Di-n-butylamine      | -3.2400 | -2.0734         | -2.1210       | -3.1400   |
| Methylacetate        | -3.1300 | -2.3746         | -2.7153       | -2.8900   |
| Methylisopropylether | -2.0100 | -1.9400         | -1.9338       | -2.1500   |
| methylether          | -1.9000 | -1.1687         | -.9355        | -1.2200   |
| Dimethyldisulfide    | -1.8300 | -1.0900         | -.7931        | -1.1100   |
| diethylsulfide       | -1.6000 | -.9890          | -1.0908       | -1.3300   |
| dimethylsulfide      | -1.5400 | -1.2394         | -1.0162       | -1.2500   |
| methylethylsulfide   | -1.5000 | -1.2242         | -1.4108       | -1.2800   |
| Di-n-propylsulfide   | -1.2800 | .1839           | .0742         | -0.5300   |
| methylsulfide        | -1.2400 | -.8549          | -.7136        | -0.8300   |
| Methanethiol         | -1.2400 | -.7571          | -.7654        | -0.8300   |
| Di-n-propylether     | -1.1600 | -.4394          | -.5721        | -1.3300   |
| n-Butanethiol        | -0.9900 | -.5538          | -.433         | -0.4800   |
| toluene              | -0.8900 | -0.164          | -0.8455       | -0.2600   |
| benzene              | -0.8700 | 0.3703          | 0.1731        | -0.3700   |
| ethylbenzene         | -0.8000 | 0.4713          | 0.7288        | -0.1600   |
| hydrogensulfide      | -0.4400 | -.2613          | -.16422       | -0.6800   |
| ethane               | 1.8300  | 1.9705          | 2.0528        | 1.8200    |
| methane              | 1.9900  | 1.822           | 1.7731        | 1.7300    |
| n-butane             | 2.0800  | 2.6302          | 2.6678        | 2.2300    |
| 22-Dimethylbutane    | 2.5100  | 3.9938          | 3.2874        | 2.8500    |
| n-Octane             | 2.8800  | 3.2461          | 3.92528       | 3.4400    |
| propane              | 1.9600  | 2.4021          | 2.1469        | 2.0600    |

TABLE XI: Hydration Free energies values in  $\text{kcal.mol}^{-1}$  from Figure 6.

## VII. THE ALANINE DIPEPTIDE

### A. Simulation Parameters

All simulations for the alanine dipeptide were performed at 298.15 K during 25 ns in a cubic box with a side length of 30 Å. The Smooth Particle Mesh Ewald method was employed with a real-space cutoff of 7 Å, and the van der Waals interactions cutoff was set at 9 Å. A BAOAB integrator with a timestep of 0.2 fs was used to accurately account for NQE. PIMD simulations were conducted with 32 beads and a friction coefficient of  $\gamma = 1 \text{ ps}^{-1}$ , while the adQTB simulations utilized a friction coefficient of  $\gamma = 20 \text{ ps}^{-1}$ .

### B. Colvar Input File

```
colvarsTrajFrequency    500
colvarsRestartFrequency 500
colvar {
  name phi
  width 5.0
  dihedral {
    oneSiteTotalForce
    group1 {
      atomnumbers 5}
    group2 {
      atomnumbers 7}
    group3 {
      atomnumbers 9}
    group4 {
      atomnumbers 15}}
    outputAppliedForce
  }
colvar {
  name psi
  width 5.0
  dihedral {
    oneSiteTotalForce
    group1 {
      atomnumbers 17}
    group2 {
      atomnumbers 15}
    group3 {
      atomnumbers 9}
    group4 {
      atomnumbers 7}}
    outputAppliedForce
  }
abf {
  colvars      phi psi
  fullSamples  500
}
```

### C. adQTB and PIMD 2D Potential of Mean Force

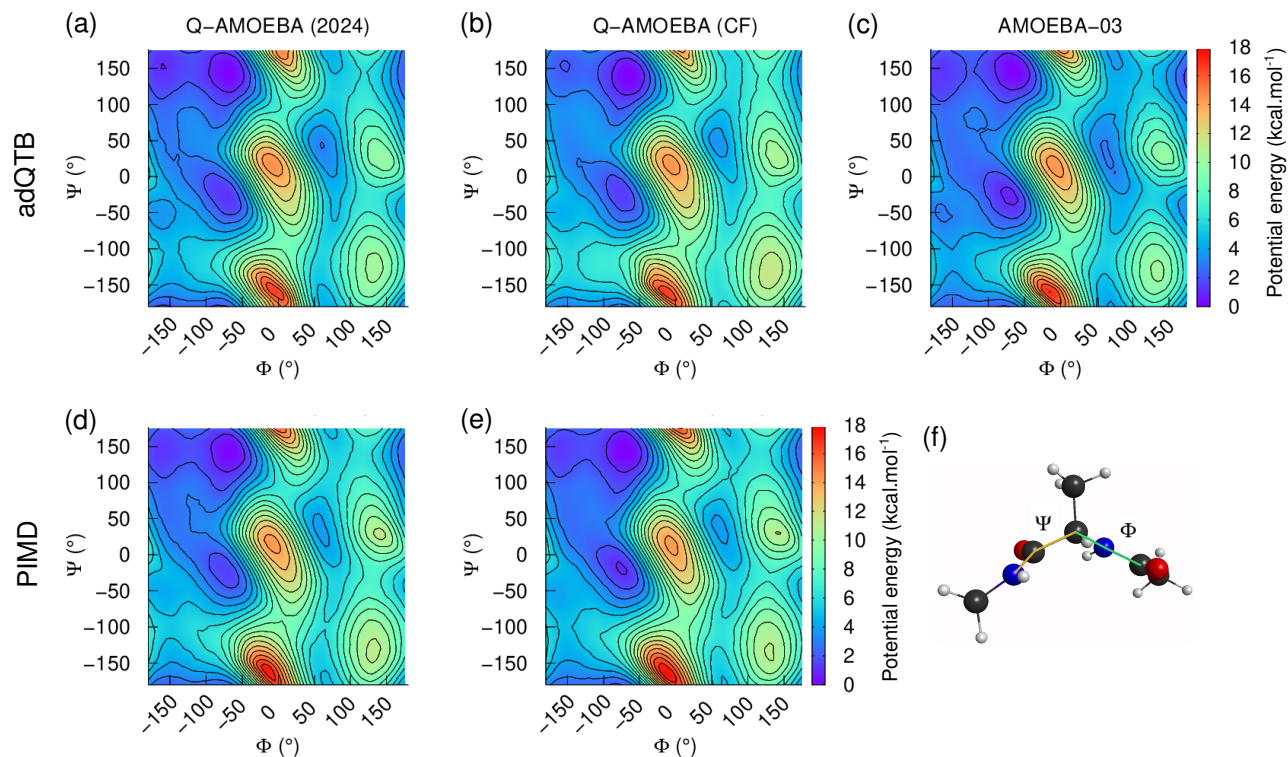

FIG. 7: Potential of Mean Force (PMF) of alanine dipeptide solvated in Q-AMOEBA (2024) (first column), Q-AMOEBA (CF) (second column), and AMOEBA-03 (third column) using the adQTB (first row) and PIMD (second row) parameter sets. The alanine dipeptide, with  $\Psi$  and  $\Phi$  angles, is illustrated in (f).

### D. PMF difference between adQTB and PIMD parameters

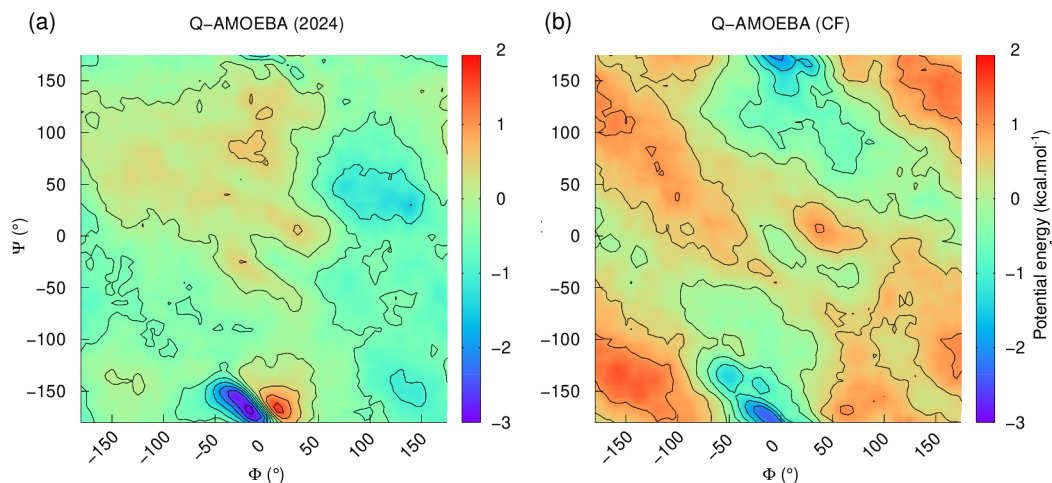

FIG. 8:  $\text{PMF}_{\text{adQTB}} - \text{PMF}_{\text{PIMD}}$  for (a) Q-AMOEBA (2024) and (b) Q-AMOEBA (CF).

### E. PMF difference between H<sub>2</sub>O and D<sub>2</sub>O solvents with adQTB

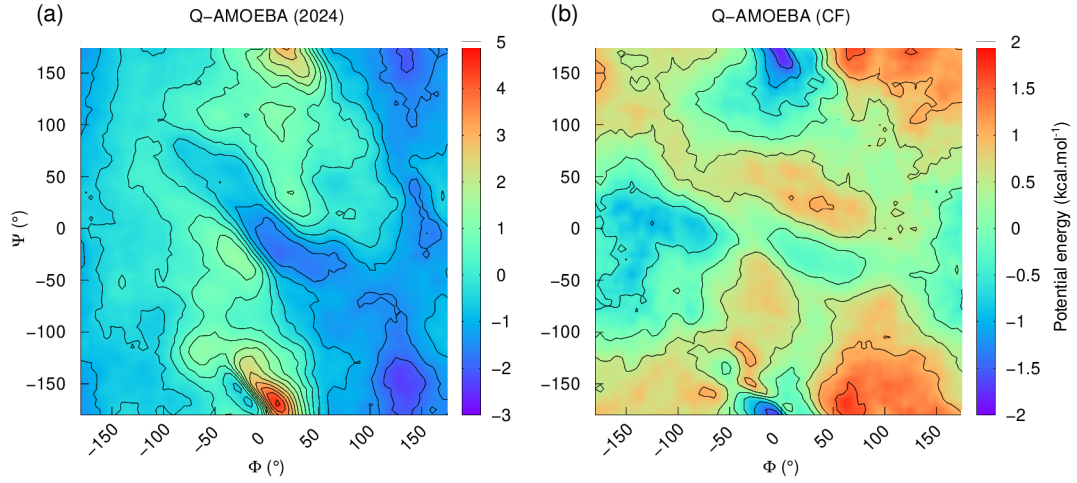

FIG. 9:  $\text{PMF}_{\text{H}_2\text{O}} - \text{PMF}_{\text{D}_2\text{O}}$  for (a) Q-AMOEBA (2024) and (b) Q-AMOEBA (CF) using parameters optimized through the adQTB method.

### F. $\lambda$ -ABF Curves of the different components in the Solvation Free Energy

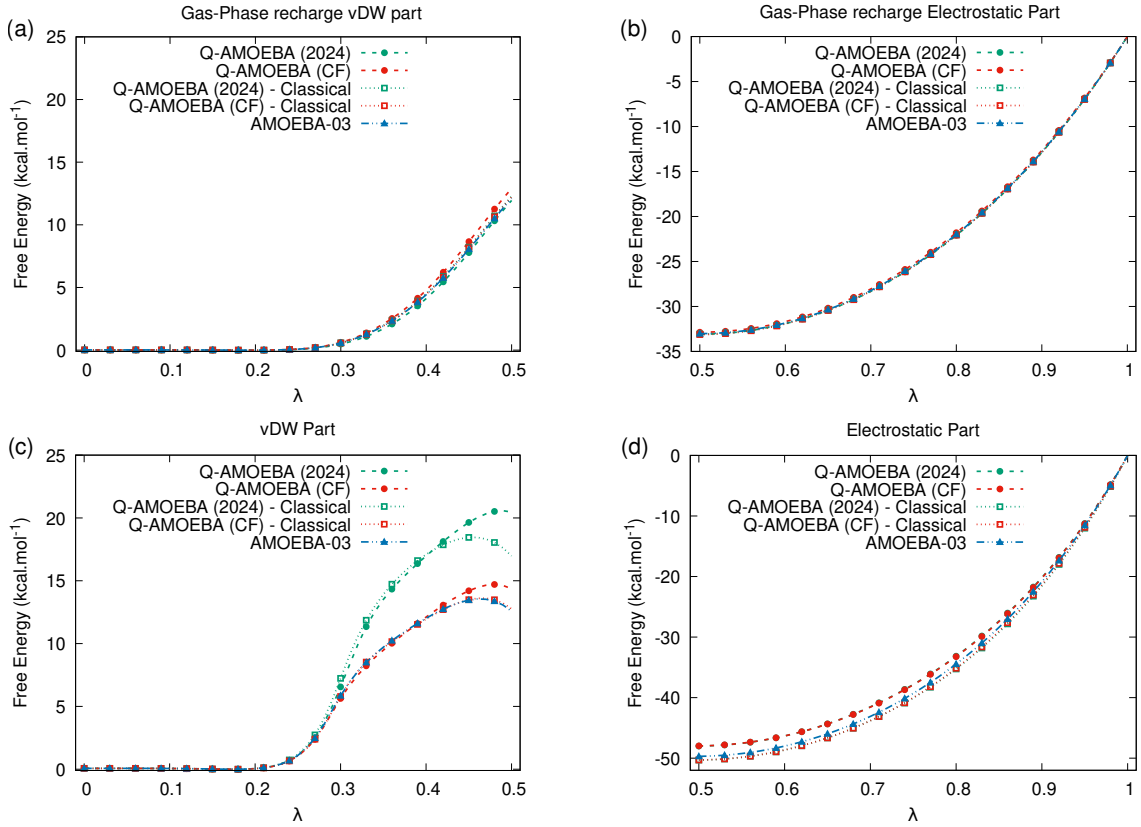

FIG. 10:  $\lambda$ -ABF curves of the different components used to computed the solvation free energy using Q-AMOEBA (2024) and Q-AMOEBA (CF) using the adQTB method with their classical counterparts and AMOEBA-03.

### G. Solvation Free Energy Decomposition

|                             | Gas-Phase Electrostatic | Electrostatic | Gas-Phase vdW | vdW     |
|-----------------------------|-------------------------|---------------|---------------|---------|
| Q-AMOEBA (2024)             | -33.0809                | -48.0008      | 11.9454       | 20.466  |
| Q-AMOEBA (CF)               | -32.8625                | -47.9755      | 12.9050       | 14.3653 |
| Q-AMOEBA (2024) - Classical | -33.0575                | -50.3124      | 12.2860       | 16.9771 |
| Q-AMOEBA (CF) - Classical   | -33.1216                | -50.2983      | 12.2204       | 12.7662 |
| AMOEBA-03                   | -33.0173                | -49.6940      | 12.1049       | 12.5778 |

TABLE XII: Various components of the hydration free energy used to compute the final solvation free energy in Table XIII.

### H. Solvation Free Energy

|                             | Solvation Free Energies |
|-----------------------------|-------------------------|
| Q-AMOEBA (2024)             | -6.407                  |
| Q-AMOEBA (CF)               | -13.65                  |
| Q-AMOEBA (2024) - Classical | -12.56                  |
| Q-AMOEBA (CF) - Classical   | -16.63                  |
| AMOEBA-03                   | -16.20                  |

TABLE XIII: Solvation free energies of the alanine dipeptide with the different models in  $\text{kcal.mol}^{-1}$  using  $\lambda$ -ABF method.

- 
- [1] U. Essmann, L. Perera, M. L. Berkowitz, T. Darden, H. Lee, and L. G. Pedersen, *The Journal of chemical physics* **103**, 8577 (1995).
- [2] P. Ren and J. W. Ponder, *The Journal of Physical Chemistry B* **107**, 5933 (2003).
- [3] N. Mauger, T. Plé, L. Lagardère, S. Huppert, and J.-P. Piquemal, *The Journal of Physical Chemistry B* **126**, 8813 (2022).
- [4] A. Soper, *Chemical Physics* **258**, 121 (2000).
- [5] W. S. Benedict, N. Gailar, and E. K. Plyler, *The Journal of Chemical Physics* **24**, 1139 (1956).
- [6] W. L. Jorgensen and C. Jenson, *Journal of Computational Chemistry* **19**, 1179 (1998).
- [7] D. M. Bates and G. S. Tschumper, *J Phys Chem A* **113**, 3555 (2009).
- [8] P. Ren and J. W. Ponder, *The Journal of Physical Chemistry B* **107**, 5933 (2003).
- [9] S. S. Xantheas and E. Aprà, *The Journal of Chemical Physics* **120**, 823 (2004).
- [10] S. Yoo, E. Aprà, X. C. Zeng, and S. S. Xantheas, *The Journal of Physical Chemistry Letters* **1**, 3122 (2010).
- [11] G. S. Fanourgakis, E. Aprà, and S. S. Xantheas, *The Journal of Chemical Physics* **121**, 2655.
- [12] L. B. Skinner, C. Huang, D. Schlesinger, L. G. M. Pettersson, A. Nilsson, and C. J. Benmore, *The Journal of Chemical Physics* **138**, 074506 (2013).
- [13] J. E. Bertie, M. K. Ahmed, and H. H. Eysel, *The Journal of Physical Chemistry* **93**, 2210 (1989).
- [14] G. S. Kell, *Journal of Chemical & Engineering Data* **20**, 97 (1975).
- [15] W. Wagner and A. Pruß, *Journal of Physical and Chemical Reference Data* **31**, 387 (2002).
- [16] G. S. Kell, *Journal of Chemical and Engineering data* **20**, 97 (1975).
- [17] S. A. Clough, Y. Beers, G. P. Klein, and L. S. Rothman, *The Journal of Chemical Physics* **59**, 2254 (1973).
- [18] Y. Badyal, M.-L. Saboungi, D. Price, S. Shastri, D. Haefner, and A. Soper, *The Journal of Chemical Physics* **112**, 9206 (2000).
- [19] P. L. Silvestrelli and M. Parrinello, *Physical Review Letters* **82**, 3308 (1999).
- [20] R. Guzzi, L. Sportelli, C. La Rosa, D. Milardi, and D. Grasso, *The Journal of Physical Chemistry B* **102**, 1021 (1998).
- [21] G. S. Kell, *Journal of Physical and Chemical Reference Data* **6**, 1109 (1977).
- [22] C. McBride, C. Vega, E. G. Noya, R. Ramírez, and L. M. Sesé, *The Journal of chemical physics* **131** (2009).
- [23] C. H. Bennett, *Journal of Computational Physics* **22**, 245 (1976).
- [24] T. Plé, N. Mauger, O. Adjoua, T. J. Inizan, L. Lagardère, S. Huppert, and J.-P. Piquemal, *Journal of Chemical Theory and Computation* **19**, 1432 (2023).
- [25] A. Grossfield, P. Ren, and J. W. Ponder, *Journal of the American Chemical Society* **125**, 15671 (2003).
- [26] R. Schmid, A. M. Miah, and V. N. Sapunov, *Phys. Chem. Chem. Phys.* **2**, 97 (2000).
